# Supplementary material for: Adaptive manifold for imbalanced transductive few-shot learning
Source: arXiv:2304.14281 source file (2023-04-27)
Supplement: Supplementary file 1 [file supp.tex]

\clearpage

% COMMENT OUT \maketitle FROM main.tex FOR \maketitle TO WORK HERE
\maketitle
\subsection{Balanced transductive few-shot learning}
Using code from \url{https://github.com/MichalisLazarou/iLPC}
%-------------------------------------------------------------------------------------------------------------------------------------------------------------------------------------------------------
\begin{table*}
\small
\centering
\setlength\tabcolsep{5pt}
\begin{tabular}{lccccccccc}
\toprule
\Th{Method}                             & \Th{Network} & \mc{2}{\Th{\emph{mini}ImageNet}}          & \mc{2}{\Th{\emph{tiered}ImageNet}}        & \mc{2}{\Th{Cifar-FS}}                     & \mc{2}{\Th{CUB}}                          \\ 
                                        &              & 1-shot              & 5-shot              & 1-shot              & 5-shot              & 1-shot              & 5-shot              & 1-shot              & 5-shot              \\ \midrule
LR+ICI~\cite{lrici}                     & \multirow{4}*{ResNet-12}   & 66.80\cip           & 79.26\cip           & 80.79\cip           & 87.92\cip           & 73.97\cip           & 84.13\cip           & 88.06\cip           & 92.53\cip           \\
% LR+ICI~\cite{lrici}*                    & ResNet-12A   & 66.85\ci{0.92}      & 78.89\ci{0.55}      & 82.40\ci{0.84}      & 88.80\ci{0.50}      & 75.36\ci{0.97}      & 84.57\ci{0.57}      & 86.53\ci{0.79}      & 92.11\ci{0.35}      \\
CAN+Top-\emph{k}~\cite{crossattention}  &     & 67.19\ci{0.55}      & 80.64\ci{0.35}      & 73.21\ci{0.58}      & 84.93 \ci{0.38}     & -                   & -                   & -                   & -                   \\
DPGN~\cite{DPGN}                        &    & 67.77\ci{0.32}      & 84.60\ci{0.43}      & 72.45\ci{0.51}      & 87.24\ci{0.39}      & 77.90\ci{0.50}      & 90.20\ci{0.40}      & 75.71\ci{0.47}      & 91.48\ci{0.33}      \\
% EP~\cite{embeddingpropagation}          & ResNet-12    & 66.50\ci{0.89}      & 81.06\ci{0.60}      & 76.53\ci{0.87}      & 87.32\ci{0.64}      & -                   & -                   & -                   & -                   \\
MCT (instance)~\cite{mct}               &    & 78.55\ci{0.86}      & 86.03\ci{0.42}      & 82.32\ci{0.81}      & 87.36\ci{0.50}      & 85.61\ci{0.69}      & 90.03\ci{0.46}      & -                   & -                   \\
% MCT (Pair)~\cite{mct}                   & ResNet-12B   & 76.16\ci{0.89}      & 85.22\ci{0.42}      & 80.68\ci{0.89}      & 86.63\ci{0.89}      & 87.28\ci{0.70}      & 90.50\ci{0.43}      & -                   & -                   \\
% \tb{\ours (ours)}                       & ResNet-12A   & \tb{69.79}\ci{0.99} &\tb{79.58}\ci{0.55}  & \tb{83.49}\ci{0.88} &\tb{89.48}\ci{0.47}  & \tb{77.14}\ci{0.95} & \tb{85.23}\ci{0.55} & \tb{88.75}\ci{0.68} & \tb{92.74}\ci{0.35} \\
\midrule
% PT+MAP~\cite{pt_map}                    & WRN-28-10    & 82.92\ci{0.26}      & 88.82\ci{0.13}      & -                   & -                   & 87.69\ci{0.23}      & 90.68\ci{0.15}      & 91.55\ci{0.19}      & 93.99\ci{0.10}      \\
% Fine-tuning~\cite{baseline_ft}          & WRN-28-10    & 65.73\ci{0.68}      & 78.40\ci{0.52}      & 73.34\ci{0.71}      & 85.50\ci{0.50}      & 76.58\ci{0.68}      & 85.79\ci{0.50}      & -                   & -                   \\
EP~\cite{embeddingpropagation}          & \multirow{14}*{WRN-28-10}    & 70.74\ci{0.85}      & 84.34\ci{0.53}      & 78.50\ci{0.91}      & 88.36\ci{0.57}      & -                   & -                   & -                   & -                   \\
SIB~\cite{SIB}$\dagger$                 &     & 70.00\ci{0.60}      & 79.20\ci{0.40}      & 72.90\cip           & 82.80\cip           & 80.00\ci{0.60}      & 85.3\ci{0.40}       & -                   & -                   \\
% DPGN~\cite{DPGN}                        & WRN-28-10    & 67.24\ci{0.51}      & 83.72\ci{0.44}      & -                   & -                   & -                   & -                   & -                   & -                   \\
SIB+E$^3$BM~\cite{ensemblefsl}          &     & 71.40\ci{0.50}      & 81.20\ci{0.40}      & 75.60\ci{0.6}       & 84.30\ci{0.4}       & -                   & -                   & -                   & -                   \\
%\tb{\ours (ours)}                       & WRN-28-10    & \tb{83.43}\ci{0.79} & \tb{89.10}\ci{0.42} & \tb{88.50}\ci{0.77} & \tb{92.99}\ci{0.42} & \tb{87.57}\ci{0.78} & \tb{91.26}\ci{0.46} & \tb{91.53}\ci{0.59} & \tb{94.27}\ci{0.30} \\ \bottomrule
LaplacianShot~\cite{laplacianshot} &  & 74.86\ci{0.19} & 84.13\ci{0.14} & 80.18\ci{0.21} & 87.56\ci{0.15} & - &- & -& -\\
PT+MAP~\cite{pt_map}                   &     & 82.88\ci{0.73}      & 88.78\ci{0.40}      & 88.15\ci{0.71}      & 92.32\ci{0.40}      & 86.91\ci{0.72}      & 90.50\ci{0.49}      & 91.37\ci{0.61}      & 93.93\ci{0.32}      \\
\ilpc~\cite{ilpc}      &     & 83.05\ci{0.79} & 88.82\ci{0.42} & 88.50\ci{0.75} & 92.46\ci{0.42} & 86.51\ci{0.75} & 90.60\ci{0.48} & 91.03\ci{0.63} & 94.11\ci{0.30}\\
EASE+SIAMESE~\cite{ease}      &     & 83.00\ci{0.21} & 88.92\ci{0.13} & 88.96\ci{0.23} & 92.63\ci{0.13} & 87.60\ci{0.23} & 90.60\ci{0.16} & 91.68\ci{0.19} & 94.12\ci{0.09}\\
TIM \cite{TIM}      &     & 77.8\cip & 87.4\cip  & 82.1\cip & 89.8\cip & - & - & - & -\\
TIM* \cite{TIM}     &     & 77.65\ci{0.72} & 88.21\ci{40}  & 83.88\ci{0.74} & 91.89\ci{0.41} & 82.63\ci{0.70} & 90.28\ci{0.46} & 87.50\ci{0.62} & 93.59\ci{0.30}\\
TIM*+PLC \cite{TIM} &     & 75.77\ci{0.67} & 88.37\ci{0.40}  & 83.22\ci{0.70} & 92.13\ci{0.40} & 80.52\ci{0.70} & 90.25\ci{0.46} & 85.58\ci{0.61} & 93.48\ci{0.31}\\
\ours ($\beta=0.8, K=20$)    &     & 80.83\ci{0.81} & 87.73\ci{0.42}  & 86.39\ci{0.77} & 91.67\ci{0.43} & 86.18\ci{0.74} & 90.14\ci{0.47} & 90.34\ci{0.68} & 93.47\ci{0.31}\\
\ours($\beta=0.9, K=10$) &    & 79.68\ci{0.78} & 87.64\ci{0.42}  & 85.62\ci{0.76} & 91.74 & 84.99\ci{0.73} & 90.17\ci{0.46} & 89.64\ci{0.66} & 93.43\ci{0.31}\\
\ours+PLC ($\beta=0.8, K=20$)    &    & 82.89\ci{0.72} & 89.03\ci{0.40}  & 88.07\ci{0.72} & 92.47\ci{0.40} & 86.81\ci{0.74} & 90.73\ci{0.46} & 91.11\ci{0.62} & 94.15\ci{0.29}\\
i\ours+PLC ($\beta=0.8, K=20$)    &    & 82.83\ci{0.82} & -  & 88.09\ci{0.77} & - & 86.63\ci{0.79} & - & 91.05\ci{0.66} & -\\
\ours+PLC($\beta=0.9, K=10$) &     & 81.52\ci{0.72} & 89.03\ci{0.40}  & 87.39\ci{0.71} & 92.49\ci{0.39} & 85.49\ci{0.72} & 90.76\ci{0.46} & 90.46\ci{0.60} & 94.08\ci{0.29}\\
\bottomrule
\end{tabular}
\vspace{6pt}
\caption{\emph{Balanced transductive inference state of the art}. *: our reproduction with official code on our datasets. $\dagger$: \emph{tiered}ImageNet as reported by~\cite{ensemblefsl}.}
\label{tab:soa-trans}
\end{table*}
%---------------------------------------------------------------------------------------------------------------------------------------------------------------------------------------------------------

\section{Original tables transferred from main}
%-----------------------------------------------------------------------------------------------------------------------------------------------------------------------------------
\begin{table*}
\small
\centering
% \begin{adjustbox}{width=1\coluwidth}
\setlength\tabcolsep{5pt}
\begin{tabular}{lcccccc}
\toprule
\Th{Method}                             & \Th{Network} & \Th{Setting} & \mc{2}{\Th{\emph{mini}ImageNet}}  & \mc{2}{\Th{\emph{tiered}ImageNet}}         \\ 
                                        &             &     & 1-shot              & 5-shot & 1-shot              & 5-shot               \\ \midrule
%Protonet~\cite{prototypical}            &  \multirow{4}*{ResNet-18}  &  \multirow{4}*{Inductive} & 53.4     & 74.2 &  -    & -       \\
%Baseline~\cite{closerlook}              &     &    & 56.0     & 78.9   & 63.5     & 83.8          \\
%Baseline++~\cite{closerlook}            &    &    & 60.4     & 79.7 & 68.0     & 84.2           \\
%Simpleshot~\cite{simpleshot}            &    &   & 63.0     & 80.1  & 69.6     & 84.7          \\
%\midrule
%MAML \cite{MAML}                         &  \multirow{11}*{ResNet-18}  &  \multirow{11}*{Transductive} & 47.6     & 64.5   & -     & -     \\
%Versa~\cite{versa}                                   &     &    & 47.8     & 61.9   & -     & -          \\
Entropy-min~\cite{entropy-min}           &    &    & 58.5     & 74.8    & 61.2     & 75.5           \\
LR+ICI~\cite{lrici}                      &    &    & 58.7     & 73.5    &  74.6    &   85.1        \\
PT-MAP~\cite{pt_map}                     &    &   & 60.1     & 67.1   & 64.1     & 70.0          \\
LaplacianShot~\cite{laplacianshot}       &    &   & 65.4     & 81.6   & 72.3     & 85.7          \\
BD-CSPN~\cite{BDCSPN}             &    &   & 67.0     & 80.2   & 74.1     & 84.8         \\
TIM~\cite{TIM}                           &    &   & 67.3     & 79.8   & 74.1     & 84.1        \\
$\alpha$-TIM~\cite{alphaTIM}             &    &   & 67.4     & 82.5    & 74.4    & 86.6        \\
$\alpha$-TIM*~\cite{alphaTIM}            &    &   & 67.15\ci{0.28}     & 82.53\ci{0.17}    & 74.34\ci{0.28}     & 86.68\ci{0.18}        \\
PLC+$\alpha$-TIM*~\cite{alphaTIM}            &    &   & 63.38\ci{0.24}     &   82.80\ci{0.17}   & 70.17\ci{0.26}     & 86.82\ci{0.18}      \\
%------------------------------------------------------OFFICIAL DATA WITH THE 2 VARIATIONS---------------------------------------------------------
% \ours($\beta=0.8, k=20$)              &    &   & 70.03\ci{0.30}     & 82.12\ci{0.17}   & 77.28\ci{0.30}     & 86.59\ci{0.18}         \\  
% \ours($\beta=0.9, k=10$)               &    &   & 68.44\ci{0.29}     & 82.41\ci{0.17}   & 75.73\ci{0.29}     & 87.02\ci{0.18}         \\ 
% PLC+\ours($\beta=0.8, k=20$)              &    &   & 70.03\ci{0.29}     & 82.75\ci{0.17}   & 76.59\ci{0.29}      & 86.72\ci{0.17}         \\
% PLC+\ours($\beta=0.9, k=10$)             &    &   & 68.99\ci{0.29}     & 83.27\ci{0.17}   & 75.75\ci{0.28}    & 87.28\ci{0.17}         \\
%--------------------------------------------------------------------------------------------------------------------------------------------------
$\alpha$-\ours                               &    &   & \tb{70.03}\ci{0.30}     & 82.41\ci{0.17}   & \tb{77.28}\ci{0.30}     & 87.02\ci{0.18}         \\  
PLC+$\alpha$-\ours                            &    &   &  \tb{70.03}\ci{0.29}     & \tb{83.27}\ci{0.17}   & 76.59\ci{0.29}   & \tb{87.28}\ci{0.17}         \\ 
\midrule
% Protonet~\cite{prototypical}            &  \multirow{4}*{WRN-28-10}  &  \multirow{4}*{Inductive} & -     & - & -     & -       \\
% Baseline~\cite{closerlook}              &     &    & 62.2     & 81.9   & 63.5      & 83.8          \\
% Baseline++~\cite{closerlook}            &    &    & 64.5     & 82.1 & 68.0     & 84.2           \\
% Simpleshot~\cite{simpleshot}            &    &   & 66.2     & 82.4  & 69.6     & 84.7          \\
% \midrule
% MAML \cite{MAML}                         &  \multirow{11}*{WRN-28-10}  &  \multirow{11}*{Transdutive} & -     & -   & -     & -     \\
% Versa                                    &     &    & -     & -   & -     & -          \\
Entropy-min \cite{entropy-min}          & \multirow{12}*{WRN-28-10}  &  \multirow{12}*{Transductive}& 60.4    & 76.2 & 62.9     & 77.3           \\
% LR+ICI~\cite{lrici}                      &    &    & -     & - & -     & -           \\
PT-MAP~\cite{pt_map}                     &    &   & 60.6     & 66.8   & 65.1     & 71.0         \\
LaplacianShot~\cite{laplacianshot}       &    &   & 68.1     & 83.2   & 73.5     & 86.8         \\
BD-CSPN~\cite{BDCSPN}             &    &   & 70.4     & 82.3   &  75.4    & 85.9         \\
TIM~\cite{TIM}                           &    &   & 69.8     & 81.6    & 75.8    & 85.4        \\
$\alpha$-TIM~\cite{alphaTIM}             &    &   & 69.8     & 84.8     & 76.0   & 87.8        \\
$\alpha$-TIM*~\cite{alphaTIM}            &    &   & 70.32\ci{0.28}     & 84.91\ci{0.16}    & 75.97\ci{0.28}     & 87.75\ci{0.18}        \\
PLC+$\alpha$-TIM*~\cite{alphaTIM}            &    &   & 66.50\ci{0.24}     & 85.12\ci{0.16}    & 71.97\ci{0.25}     &  88.28\ci{0.16}      \\
% \ours($\beta=0.8, k=20$)              &    &   & 72.54\ci{0.29}     & 84.17\ci{0.16}   & 78.90\ci{0.30}     & 87.63\ci{0.17}         \\  
% \ours($\beta=0.9, k=10$)               &    &   & 71.21\ci{0.29}     & 84.71\ci{0.16}   & 77.25\ci{0.29}     & 88.05\ci{0.17}        \\ 
% PLC+\ours($\beta=0.8, k=20$)              &    &   & 71.55\ci{0.29}     & 84.78\ci{0.16}   & 78.66\ci{0.29}     & 88.01\ci{0.17}         \\
% PLC+\ours($\beta=0.9, k=10$)             &    &   & 71.48\ci{0.28}     & 85.71\ci{0.16}   & 77.90\ci{0.27}     & 88.67\ci{0.17}         \\  
$\alpha$-\ours                        &    &   & \tb{72.54}\ci{0.29}     & 84.71\ci{0.16}   & \tb{78.90}\ci{0.30}     & 88.05\ci{0.17}        \\  
PLC+$\alpha$-\ours                       &    &   & 71.55\ci{0.29}     & \tb{85.71}\ci{0.16}   & 78.66\ci{0.29}     & \tb{88.67}\ci{0.17}        \\

\bottomrule
\end{tabular}
% \end{adjustbox}
\vspace{6pt}
\caption{\emph{Imbalanced transductive inference experimental comparisons with state of the art}. The results are reported as provided from \cite{alphaTIM}. *: our reproduction with official code using the publicly available code provided from \cite{alphaTIM}. $\dagger$: \emph{tiered}ImageNet as reported by~\cite{ensemblefsl}.}
\label{tab:soa-trans}
\end{table*}
%--------------------------------------------------------------------------------------------------------------------------------------------------------------------------------

%--------------------------------------------------------------------------------------------------------------------------------------------------------------------------------------
\begin{table*}
\small
\centering
% \begin{adjustbox}{width=1\coluwidth}
\setlength\tabcolsep{5pt}
\begin{tabular}{lcccccc}
\toprule
\Th{Method}                             & \Th{Network} & \Th{Setting} & \mc{2}{\Th{\emph{mini}ImageNet}}  & \mc{2}{\Th{\emph{tiered}ImageNet}}         \\ 
                                        &             &     & 1-shot              & 5-shot & 1-shot              & 5-shot               \\ \midrule
Protonet~\cite{prototypical}            &  \multirow{4}*{ResNet-18}  &  \multirow{4}*{Inductive} & 56.10\ci{0.20}    & 78.72\ci{0.15}   & 63.28\ci{0.23}    & 84.10\ci{0.16}         \\
Baseline~\cite{closerlook}              &     &    & 56.10\ci{0.20}    & 78.80\ci{0.14}   & 63.28\ci{0.23}    & 84.12\ci{0.16}         \\
Baseline++~\cite{closerlook}            &    &    & 60.22\ci{0.20}    & 79.72\ci{0.14}   & 68.06\ci{0.22}    & 84.50\ci{0.15}         \\
Simpleshot~\cite{simpleshot}            &    &   & 63.00\ci{0.20}    & 80.09\ci{0.14}   & 69.72\ci{0.22}    & 84.87\ci{0.15}         \\
\midrule
Entropy-min~\cite{entropy-min}           &  \multirow{11}*{ResNet-18}  &  \multirow{11}*{Transductive} & -    & -   & -    & -         \\
PT-MAP~\cite{pt_map}                     &    &   & 76.88\ci{0.27}    & 85.18\ci{0.14}   & 82.89\ci{0.26}    & 88.64\ci{0.15}         \\
LaplacianShot~\cite{laplacianshot}       &    &   & 70.24\ci{0.23}    & 82.10\ci{0.14}   & 77.28\ci{0.24}    & 86.22\ci{0.16}         \\
BD-CSPN~\cite{BDCSPN}             &    &   & 69.36\ci{0.23}    & 82.06\ci{0.14}   & 76.36\ci{0.24}    & 86.18\ci{0.16}         \\
TIM~\cite{TIM}                           &    &   & 73.81\ci{0.25}    & 84.91\ci{0.15}   & 80.13\ci{0.25}    & 88.61\ci{0.15}         \\
PLC+TIM*~\cite{TIM}            &    &   & 69.33\ci{0.23}    & 84.53\ci{0.14}   & 76.36\ci{0.24}    & 88.33\ci{0.15}         \\
\ours($\beta=0.8, k=20$)              &    &   & 76.37\ci{0.28}    & 84.85\ci{0.15}   &  82.68\ci{0.27}    & 88.29\ci{0.16}         \\ 
\ours($\beta=0.9, k=10$)               &    &   & 74.87\ci{0.27}    & 84.80\ci{0.15}   & 81.70\ci{0.26}    & 88.60\ci{0.15}         \\
PLC+\ours($\beta=0.8, k=20$)              &    &   & 77.46\ci{0.27}    & 85.25\ci{0.14}   & 83.53\ci{0.26}    & 88.85\ci{0.15}         \\
PLC+\ours($\beta=0.9, k=10$)             &    &   & 75.84\ci{0.26}    & \tb{85.47}\ci{0.14}   & 82.17\ci{0.25}    & 89.06\ci{0.15}         \\
\midrule
Protonet~\cite{prototypical}            &  \multirow{4}*{WRN-28-10}  &  \multirow{4}*{Inductive} & 60.87\ci{0.20}     & 81.52\ci{0.14} & 64.59\ci{0.23}     & 84.95\ci{0.16}       \\
Baseline~\cite{closerlook}              &     &    & 60.87\ci{0.20}    & 81.61\ci{0.14}   & 64.59\ci{0.23}    & 84.97\ci{0.16}         \\
Baseline++~\cite{closerlook}            &    &    & 63.10\ci{0.20}    & 82.02\ci{0.14}   & 68.58\ci{0.22}    & 85.43\ci{0.15}         \\
Simpleshot~\cite{simpleshot}            &    &   &  65.76\ci{0.20}    & 82.27\ci{0.14}   & 70.77\ci{0.22}    & 85.81\ci{0.15}         \\
\midrule
Entropy-min \cite{entropy-min}          & \multirow{12}*{WRN-28-10}  &  \multirow{12}*{Transductive} & -    & -   & -    & -         \\
PT-MAP~\cite{pt_map}                     &    &   & 80.35\ci{0.25}    & 87.37\ci{0.13}   & 84.84\ci{0.25}    & 89.86\ci{0.15}         \\
LaplacianShot~\cite{laplacianshot}       &    &   & 72.91\ci{0.23}    & 83.85\ci{0.14}   & 78.85\ci{0.24}    & 87.27\ci{0.15}         \\ 
BD-CSPN~\cite{BDCSPN}             &    &   & 72.16\ci{0.22}    & 83.78\ci{0.14}   & 77.88\ci{0.24}    & 87.23\ci{0.15}         \\
TIM~\cite{TIM}                           &    &  & 77.78\ci{0.24}    & 87.43\ci{0.13}   & 82.28\ci{0.24}    & 89.84\ci{0.15}         \\
PLC+TIM*~\cite{TIM}            &    &  & 73.52\ci{0.22}    & 86.95\ci{0.95}   & 78.23\ci{0.24}    & 89.56\ci{0.14}         \\
\ours($\beta=0.8, k=20$)              &    &   & 79.70\ci{0.26}    & 86.91\ci{0.13}   & 84.34\ci{0.26}    & 89.36\ci{0.15}         \\ 
\ours($\beta=0.9, k=10$)               &    &   & 78.27\ci{0.26}    & 87.07\ci{0.13}   & 83.44\ci{0.25}    & 89.68\ci{0.15}         \\
PLC+\ours($\beta=0.8, k=20$)              &    &   & 81.04\ci{0.26}    & 87.61\ci{0.13}   & 85.34\ci{0.25}    & 90.06\ci{0.15}         \\
PLC+\ours($\beta=0.9, k=10$)             &    &   & 79.58\ci{0.25}    & 87.85\ci{0.13}   & 84.21\ci{0.24}    & 90.28\ci{0.14}         \\  
\bottomrule
\end{tabular}
% \end{adjustbox}
\vspace{6pt}
\caption{\emph{Balanced transductive inference experimental comparisons with state of the art}. The results are reported as provided from \cite{alphaTIM}. *: our reproduction with official code using the publicly available code provided from \cite{alphaTIM}. $\dagger$: \emph{tiered}ImageNet as reported by~\cite{ensemblefsl}.}
\label{tab:soa-trans}
\end{table*}
%-------------------------------------------------------------------------------------------------------------------------------------------------------------------------------------

%--------------------------------------------------------------------------------------------------------------------------------------------------------------------------------------
\begin{table*}
\small
\centering
% \begin{adjustbox}{width=1\coluwidth}
\setlength\tabcolsep{5pt}
\begin{tabular}{lcccc}
\toprule
\Th{Method}                             & \Th{Network} & \Th{Setting} & \mc{2}{\Th{CUB}}        \\              
    &             &     & 1-shot              & 5-shot            \\ \midrule
Protonet~\cite{prototypical}            &  \multirow{4}*{ResNet-18}  &  \multirow{4}*{Inductive} & 64.51\ci{0.21}    & 86.91\ci{0.12}        \\
Baseline~\cite{closerlook}              &     &    & 64.51\ci{0.21}    & 87.02\ci{0.11}         \\
Baseline++~\cite{closerlook}            &    &    & 69.47\ci{0.21}    & 87.63\ci{0.11}         \\
Simpleshot~\cite{simpleshot}            &    &   & 70.53\ci{0.20}    & 87.60\ci{0.11}        \\
\midrule
Entropy-min~\cite{entropy-min}          &  \multirow{8}*{ResNet-18}  &  \multirow{11}*{Transductive} & -    & -         \\
PT-MAP~\cite{pt_map}                    &    &   & 86.05\ci{0.23}    & 91.28\ci{0.11}         \\
LaplacianShot~\cite{laplacianshot}      &    &   & 79.55\ci{0.22}    & 88.96\ci{0.11}         \\
BD-CSPN~\cite{BDCSPN}                   &    &   & 78.52\ci{0.22}    & 89.02\ci{0.11}         \\
TIM~\cite{TIM}                          &    &   & 82.87\ci{0.22}     & 91.58\ci{0.10}       \\
PLC+TIM*~\cite{TIM}                     &    &   & 77.69\ci{0.22}    & 91.17\ci{0.10} \\
\ours($\beta=0.8, k=20$)                &    &   & 85.88\ci{0.24}    & 91.16\ci{0.10}        \\ 
\ours($\beta=0.9, k=10$)                &    &   & 84.30\ci{0.23}    & 91.35\ci{0.10}        \\
PLC+\ours($\beta=0.8, k=20$)            &    &   & 86.80\ci{0.23}    & 91.68\ci{0.10}        \\
PLC+\ours($\beta=0.9, k=10$)            &    &   & 85.19\ci{0.23}    & 91.86\ci{0.10}         \\
\bottomrule
\end{tabular}
% \end{adjustbox}
\vspace{6pt}
\caption{\emph{Balanced transductive inference experimental comparisons with state of the art}. The results are reported as provided from \cite{alphaTIM}. *: our reproduction with official code using the publicly available code provided from \cite{alphaTIM}. $\dagger$: \emph{tiered}ImageNet as reported by~\cite{ensemblefsl}.}
\label{tab:soa-trans_cub}
\end{table*}
%-------------------------------------------------------------------------------------------------------------------------------------------------------------------------------------

%------------------------------------------------------------------------------
\begin{table}
% \small
\centering
% \begin{adjustbox}{width=1\columnwidth}
\setlength\tabcolsep{5pt}
\begin{tabular}{lcccc}
\toprule
\Th{Method}                             & \Th{Network} & \Th{Setting} & \mc{2}{\Th{CUB}}       \\ 
                                        &             &     & 1-shot              & 5-shot         \\ \midrule
Baseline~\cite{closerlook}              &  \multirow{3}*{ResNet-18}  &  \multirow{3}*{Inductive}    & 64.6     & 86.9          \\
Baseline++~\cite{closerlook}            &    &    & 69.4     & 87.5            \\
Simpleshot~\cite{simpleshot}            &    &   & 70.6     & 87.5          \\
\midrule
PT-MAP~\cite{pt_map}                     &  \multirow{11}*{ResNet-18}  &  \multirow{11}*{Transductive} & 65.1     & 71.3      \\
Entropy-min~\cite{entropy-min}           &    &   & 67.5     & 82.9          \\
LaplacianShot~\cite{laplacianshot}       &    &   & 73.7     & 87.7           \\
BD-CSPN~\cite{BDCSPN}                   &    &   & 74.5     & 87.1           \\
TIM~\cite{TIM}                           &    &   & 74.8     & 86.9        \\
$\alpha$-TIM~\cite{alphaTIM}             &    &   & 75.7     & 89.8       \\
*$\alpha$-TIM~\cite{alphaTIM}            &    &   & 76.57\ci{0.26}     & 90.03\ci{0.12}         \\
PLC+$\alpha$-TIM*~\cite{alphaTIM}        &    &   & 70.95\ci{0.23}    & 89.56\ci{0.12}   \\
\ours($\beta=0.8, k=20$)                &    &   & 80.00\ci{0.28}     & 89.72\ci{0.12}           \\ 
PLC+\ours($\beta=0.8, k=20$)            &    &   & 79.02\ci{0.28}     & 89.62\ci{0.12}          \\ 
\ours($\beta=0.9, k=10$)                &    &   & 76.81\ci{0.28}     & 89.64\ci{0.12}           \\ 
PLC+\ours($\beta=0.9, k=10$)            &    &   & 77.03\ci{0.27}     & 89.80\ci{0.12}           \\\bottomrule

\end{tabular}
% \end{adjustbox}
\vspace{6pt}
\caption{\emph{Imbalanced transductive inference experimental comparisons with state of the art}. The results are reported as provided from \cite{alphaTIM}. *: our reproduction with official code using the publicly available code provided from \cite{alphaTIM}. $\dagger$: \emph{tiered}ImageNet as reported by~\cite{ensemblefsl}.}
\label{tab:soa-trans}
\end{table}
%------------------------------------------------------------------------------

%------------------------------------------------------------------------------
\begin{table}
\small
\centering
\begin{tabular}{lcccc}
\toprule
\Th{Method}   & \mc{2}{\Th{\emph{mini}ImageNet}}          & \mc{2}{\Th{\emph{tiered}ImageNet}} \\
           & 1-shot              & 5-shot              & 1-shot              & 5-shot\\ \midrule
                        \mc{5}{\Th{Imbalanced - ResNet-18}} \\ \midrule
$\alpha$-TIM~\cite{alphaTIM}     & 69.53\ci{0.28}     & 83.73\ci{0.16}      & 76.07\ci{0.28}    & 87.13\ci{0.18}     \\
$\alpha$-\ours              & \tb{73.68}\ci{0.29} & \tb{83.97}\ci{0.16} &  \tb{80.43}\ci{0.29} & \tb{88.32}\ci{0.16}  \\ %\midrule
    %                    \mc{5}{\Th{Balanced - ResNet-18}} \\ \midrule
%TIM~\cite{TIM}     & 76.78\ci{0.24}     & 85.82\ci{0.12}     & 82.43\ci{0.24}    &  89.09\ci{0.13}     \\
%\ours              & 79.04\ci{0.26}      & 86.04 &  - & -  \\
\bottomrule
\end{tabular}
\vspace{6pt}
\caption{\emph{Imbalanced transductive inference, 250 queries in total}}
\label{tab:trans-50q}
\end{table}
%-----------------------------------------------------------------------------

% PAGE NUMBER SET TO 1
\setcounter{page}{1}

% LINE NUMBER SET TO 1
\iccvrulercount=1

% START APPENDIX
\appendix
